# Supplementary material for: Feature Diversification and Adaptation for Federated Domain Generalization
Source: arXiv:2407.08245 source file (2024-07-11)
Supplement: Supplementary file 1 [file supple_officehome_table.tex]

\begin{table}[t]
\caption{Comparison results on OfficeHome. Gray color indicates federated DG methods posing privacy issues.}
\centering
\vspace{-2mm}
\resizebox{0.48\textwidth}{!}{
\begin{tabular}{c|cccccc}
\toprule
\multirow{2}{*}{Method} & \multicolumn{5}{c}{OfficeHome}                  \\ \cline{2-6} 
                        & A & C & P & \multicolumn{1}{c|}{R} & Avg. \\ \midrule
FedAvg~\cite{FedAvg}                  & 56.82 (0.31) & 50.53 (0.60) & 72.38 (0.24) & \multicolumn{1}{c|}{\textbf{74.16 (0.38)}} & 63.47 \\
FedProx~\cite{FedProx}                & 56.58 (0.63) & 49.44 (0.39) & 72.15 (0.30) & \multicolumn{1}{c|}{73.90 (0.46)} & 63.02 \\
FedBN~\cite{FedBN}                 & \textbf{58.31 (0.36)} & 50.07 (0.49) & 72.53 (0.70) & \multicolumn{1}{c|}{74.06 (0.50))} & 63.75 \\
SiloBN~\cite{SiloBN}         & 58.29 (0.70) & \textbf{51.16 (0.48)} & \textbf{72.80 (0.59)} & \multicolumn{1}{c|}{74.06 (0.51)} & \textbf{64.08} \\ \midrule
RandAug~\cite{RandAug}    & \textbf{58.50 (0.34)} & 52.18 (0.77) & \textbf{73.17 (0.36)} & \multicolumn{1}{c|}{\textbf{74.52 (0.52)}} & \textbf{64.59} \\
Mixstyle~\cite{Mixstyle}                & 55.57 (1.24) & 53.31 (0.65) & 70.90 (0.81) & \multicolumn{1}{c|}{73.18 (0.27)} & 63.24 \\ 
SFA~\cite{SFA}                 & 50.99 (1.20) & 50.97 (0.35) & 66.84 (0.65) & \multicolumn{1}{c|}{69.08 (0.23)} & 59.47 \\ 
RandConv~\cite{RandConv}             & 56.19 (0.80) & 53.20 (0.47) & 71.66 (0.57) & \multicolumn{1}{c|}{71.94 (0.46)} & 63.25 \\ 
L2D~\cite{L2D}       & 54.70 (1.43) & \textbf{56.36 (0.28)} & 69.96 (0.85) & \multicolumn{1}{c|}{72.13 (0.35)} & 63.29 \\ \cmidrule{1-6} 
JiGen~\cite{JiGen}                   & 58.20 (0.67)  &  50.00 (0.02) & \textbf{73.99 (0.56)}  & \multicolumn{1}{c|}{74.18 (0.00)}  &    64.09  \\
RSC~\cite{RSC}                   & 56.67 (0.59)  & 49.59 (1.05)  & 71.61 (0.47)  & \multicolumn{1}{c|}{74.16 (0.49)}  & 63.01 \\
SelfReg~\cite{SelfReg}                     &  \textbf{59.26 (0.26)} & \textbf{51.84 (0.86)} & 73.46 (0.18)  & \multicolumn{1}{c|}{\textbf{74.85 (0.62)}}  & \textbf{64.85} \\ \midrule
\cellcolor[gray]{0.9}{COPA~\cite{COPA}}                 & \cellcolor[gray]{0.9}53.39 (0.16) & \cellcolor[gray]{0.9}57.46 (0.47) & \cellcolor[gray]{0.9}68.61 (0.15) & \multicolumn{1}{c|}{\cellcolor[gray]{0.9}70.24 (0.38)} & \cellcolor[gray]{0.9}62.42  \\
\cellcolor[gray]{0.9}{FedDG~\cite{FedDG}}  & \cellcolor[gray]{0.9}59.87 (0.06) & \cellcolor[gray]{0.9}53.51 (0.31) & \cellcolor[gray]{0.9}72.81 (0.89) & \multicolumn{1}{c|}{\cellcolor[gray]{0.9}73.41 (0.41)} & \cellcolor[gray]{0.9}64.90 \\ \cmidrule{1-6} 
CSAC~\cite{CSAC}         & \textbf{58.97 (1.13)} & 51.61 (0.26) & \textbf{72.57 (0.18)} & \multicolumn{1}{c|}{74.25 (0.49)} & 64.35  \\ 
FedSR~\cite{FedSR}       & 57.59 (0.49) & 49.62 (0.91) & 72.24 (0.64) & \multicolumn{1}{c|}{74.36 (0.18)} & 63.45  \\ 
FedSAM~\cite{FedSAM}     & 55.25 (0.48) & 49.54 (0.57) & 71.07 (0.14) & \multicolumn{1}{c|}{72.77 (0.36)} & 62.16  \\ 
SiloBN w/ GA~\cite{GA}   & 58.93 (1.13) & 51.06 (0.41) & 72.42 (0.87) & \multicolumn{1}{c|}{74.36 (0.11)} & 64.19  \\ 
FedFD (ours)   &  57.68 (0.64) & 52.90 (0.13) & 71.79 (0.47) & \multicolumn{1}{c|}{73.68 (0.39)} & 64.01 \\ 
FedFD-A (ours)  &  58.62 (0.51) & \textbf{53.47 (0.21)} & 72.34 (0.45) & \multicolumn{1}{c|}{\textbf{74.39 (0.17)}} & \textbf{64.71} \\ \bottomrule
\end{tabular}
}
\label{main_table3}
\end{table}
